# Supplementary material for: MoVelo: World-Grounded Human Motion Recovery with Feedback from Conditional Velocity Field
Source: arXiv:2611.37331 source file (2026-11-27)
Supplement: Supplementary file 2 [file supp_contents.tex]

\begingroup
\iftoggle{cvprfinal}{}{\nolinenumbers}
\raggedright
\small
\renewcommand{\arraystretch}{1.06}
\newcommand{\appcontentsrow}[4][]{%
  \hyperref[#2]{#1#3\ref*{#2}} &
  \hyperref[#2]{#1#4} &
  \hyperref[#2]{\pageref*{#2}} \\
}
\noindent\pdfbookmark[0]{Supplementary Material}{supplementary-start}%
{\normalsize\bfseries Table of Contents}\par
\vspace{2pt}
\hrule
\vspace{3pt}
\noindent
\begin{minipage}[t]{\columnwidth}
\begin{tabular*}{\linewidth}[t]{@{}l@{\hspace{8pt}}l@{\extracolsep{\fill}}r@{}}
\appcontentsrow[\bfseries]{sec:app-implementation}{}{Implementation and Training Details}
\appcontentsrow{sec:app-network}{}{Network Architecture and Initialization}
\appcontentsrow{sec:app-objectives}{}{Training Objectives and Loss Weights}
\appcontentsrow{sec:app-training}{}{Training Settings}
\appcontentsrow{sec:app-evaluation}{}{Evaluation Protocols and Metrics}
\appcontentsrow[\bfseries]{sec:app-qualitative}{}{Additional Visualizations}
\appcontentsrow{fig:app-world-scene}{Fig.~}{Long-Sequence Reconstruction}
\appcontentsrow{fig:occlusion-and-truncation}{Fig.~}{Occlusion and Truncation}
\end{tabular*}
\end{minipage}\hfill
\begin{minipage}[t]{\columnwidth}
\begin{tabular*}{\linewidth}[t]{@{}l@{\hspace{8pt}}l@{\extracolsep{\fill}}r@{}}
\appcontentsrow{fig:app-cross-attention}{Fig.~}{Decoder Cross-Attention}
\appcontentsrow{fig:app-emdb2-trajectories}{Fig.~}{Human Trajectories on EMDB-2}
\appcontentsrow[\bfseries]{sec:app-quantitative}{}{Additional Experimental Results}
\appcontentsrow{sec:app-supervision-ablation}{}{Velocity Field Supervision}
\appcontentsrow{sec:app-endpoint-objective}{}{Loss on Integrated Joint Positions}
\appcontentsrow{sec:app-local-reconstruction}{}{Local Mesh Reconstruction}
\appcontentsrow{sec:app-rich-temporal}{}{Temporal Consistency on RICH}
\appcontentsrow[\bfseries]{sec:app-limitations}{}{Limitations}
\end{tabular*}
\end{minipage}\par
\vspace{3pt}
\hrule
\vspace{9pt}
\endgroup
